# Supplementary material for: Robust Non-termination Analysis of Numerical Software
Source: arXiv:1804.01391 source file (2018-10-28)
Supplement: Supplementary file 1 [file Appendix.tex]

%\section*{Appendix}
%\begin{proof}
%2. In order to prove continuity, let $\bm{x},\bm{y}\in \mathcal{R}_0$. Then 
%\begin{equation}
%\begin{split}
%|V(\bm{x}_1)-V(\bm{x}_2)|&\leq \sup_{\bm{d}\in \mathcal{D}_R}\sup_{k\in [0,+\infty)}\big(\sum_{i=0}^k|\ln(g(\bm{y}_{\bm{x}_1}^{\bm{d}}(i-1),\bm{d}_{i-1})+1)-\ln(g(\bm{y}_{\bm{x}_2}^{\bm{d}}(i-1),\bm{d}_{i-1})+1)|\\
%&+|\ln(1-h(\bm{y}_{\bm{x}_1}^{\bm{d}}(k)))-\ln(1-h(\bm{y}_{\bm{x}_2}^{\bm{d}}(k)))|\big)\\
%&\leq \sup_{\bm{d}\in \mathcal{D}_R}\sum_{i=0}^{\infty}|\ln(g(\bm{y}_{\bm{x}_1}^{\bm{d}}(i-1),\bm{d}_{i-1})+1)-\ln(g(\bm{y}_{\bm{x}_2}^{\bm{d}}(i-1),\bm{d}_{i-1})+1)|\\
%&+\sup_{\bm{d}\in \mathcal{D}_R}\sup_{k\in [0,+\infty)}|\ln(1-h(\bm{y}_{\bm{x}_1}^{\bm{d}}(k)))-\ln(1-h(\bm{y}_{\bm{x}_2}^{\bm{d}}(k)))|\\
%&\leq \sup_{\bm{d}\in \mathcal{D}_R}\sum_{i=0}^{\infty}\abs{g(\bm{y}_{\bm{x}_1}^{\bm{d}}(i-1),\bm{d}_{i-1})-g(\bm{y}_{\bm{x}_2}^{\bm{d}}(i-1),\bm{d}_{i-1})}\\
%&+M\sup_{\bm{d}\in \mathcal{D}_R}\sup_{k\in [0,+\infty)}\abs{h(\bm{y}_{\bm{x}_1}^{\bm{d}}(k))-h(\bm{y}_{\bm{x}_2}^{\bm{d}}(k))}
%\end{split}
%\end{equation}

%3. Follows immediately from (1) and (2) using the formula $v(\bm{x})=1-e^{-V(\bm{x})}$.
%\end{proof}
